# Supplementary material for: Methods for differential network estimation: an empirical comparison
Source: arXiv:2412.17922 source file (2025-03-06)
Supplement: Supplementary file 1 [file Supplementary_abc.pdf]

# Supplementary materials, Figure (a): graphs used in the simulation study

## Random differential graph

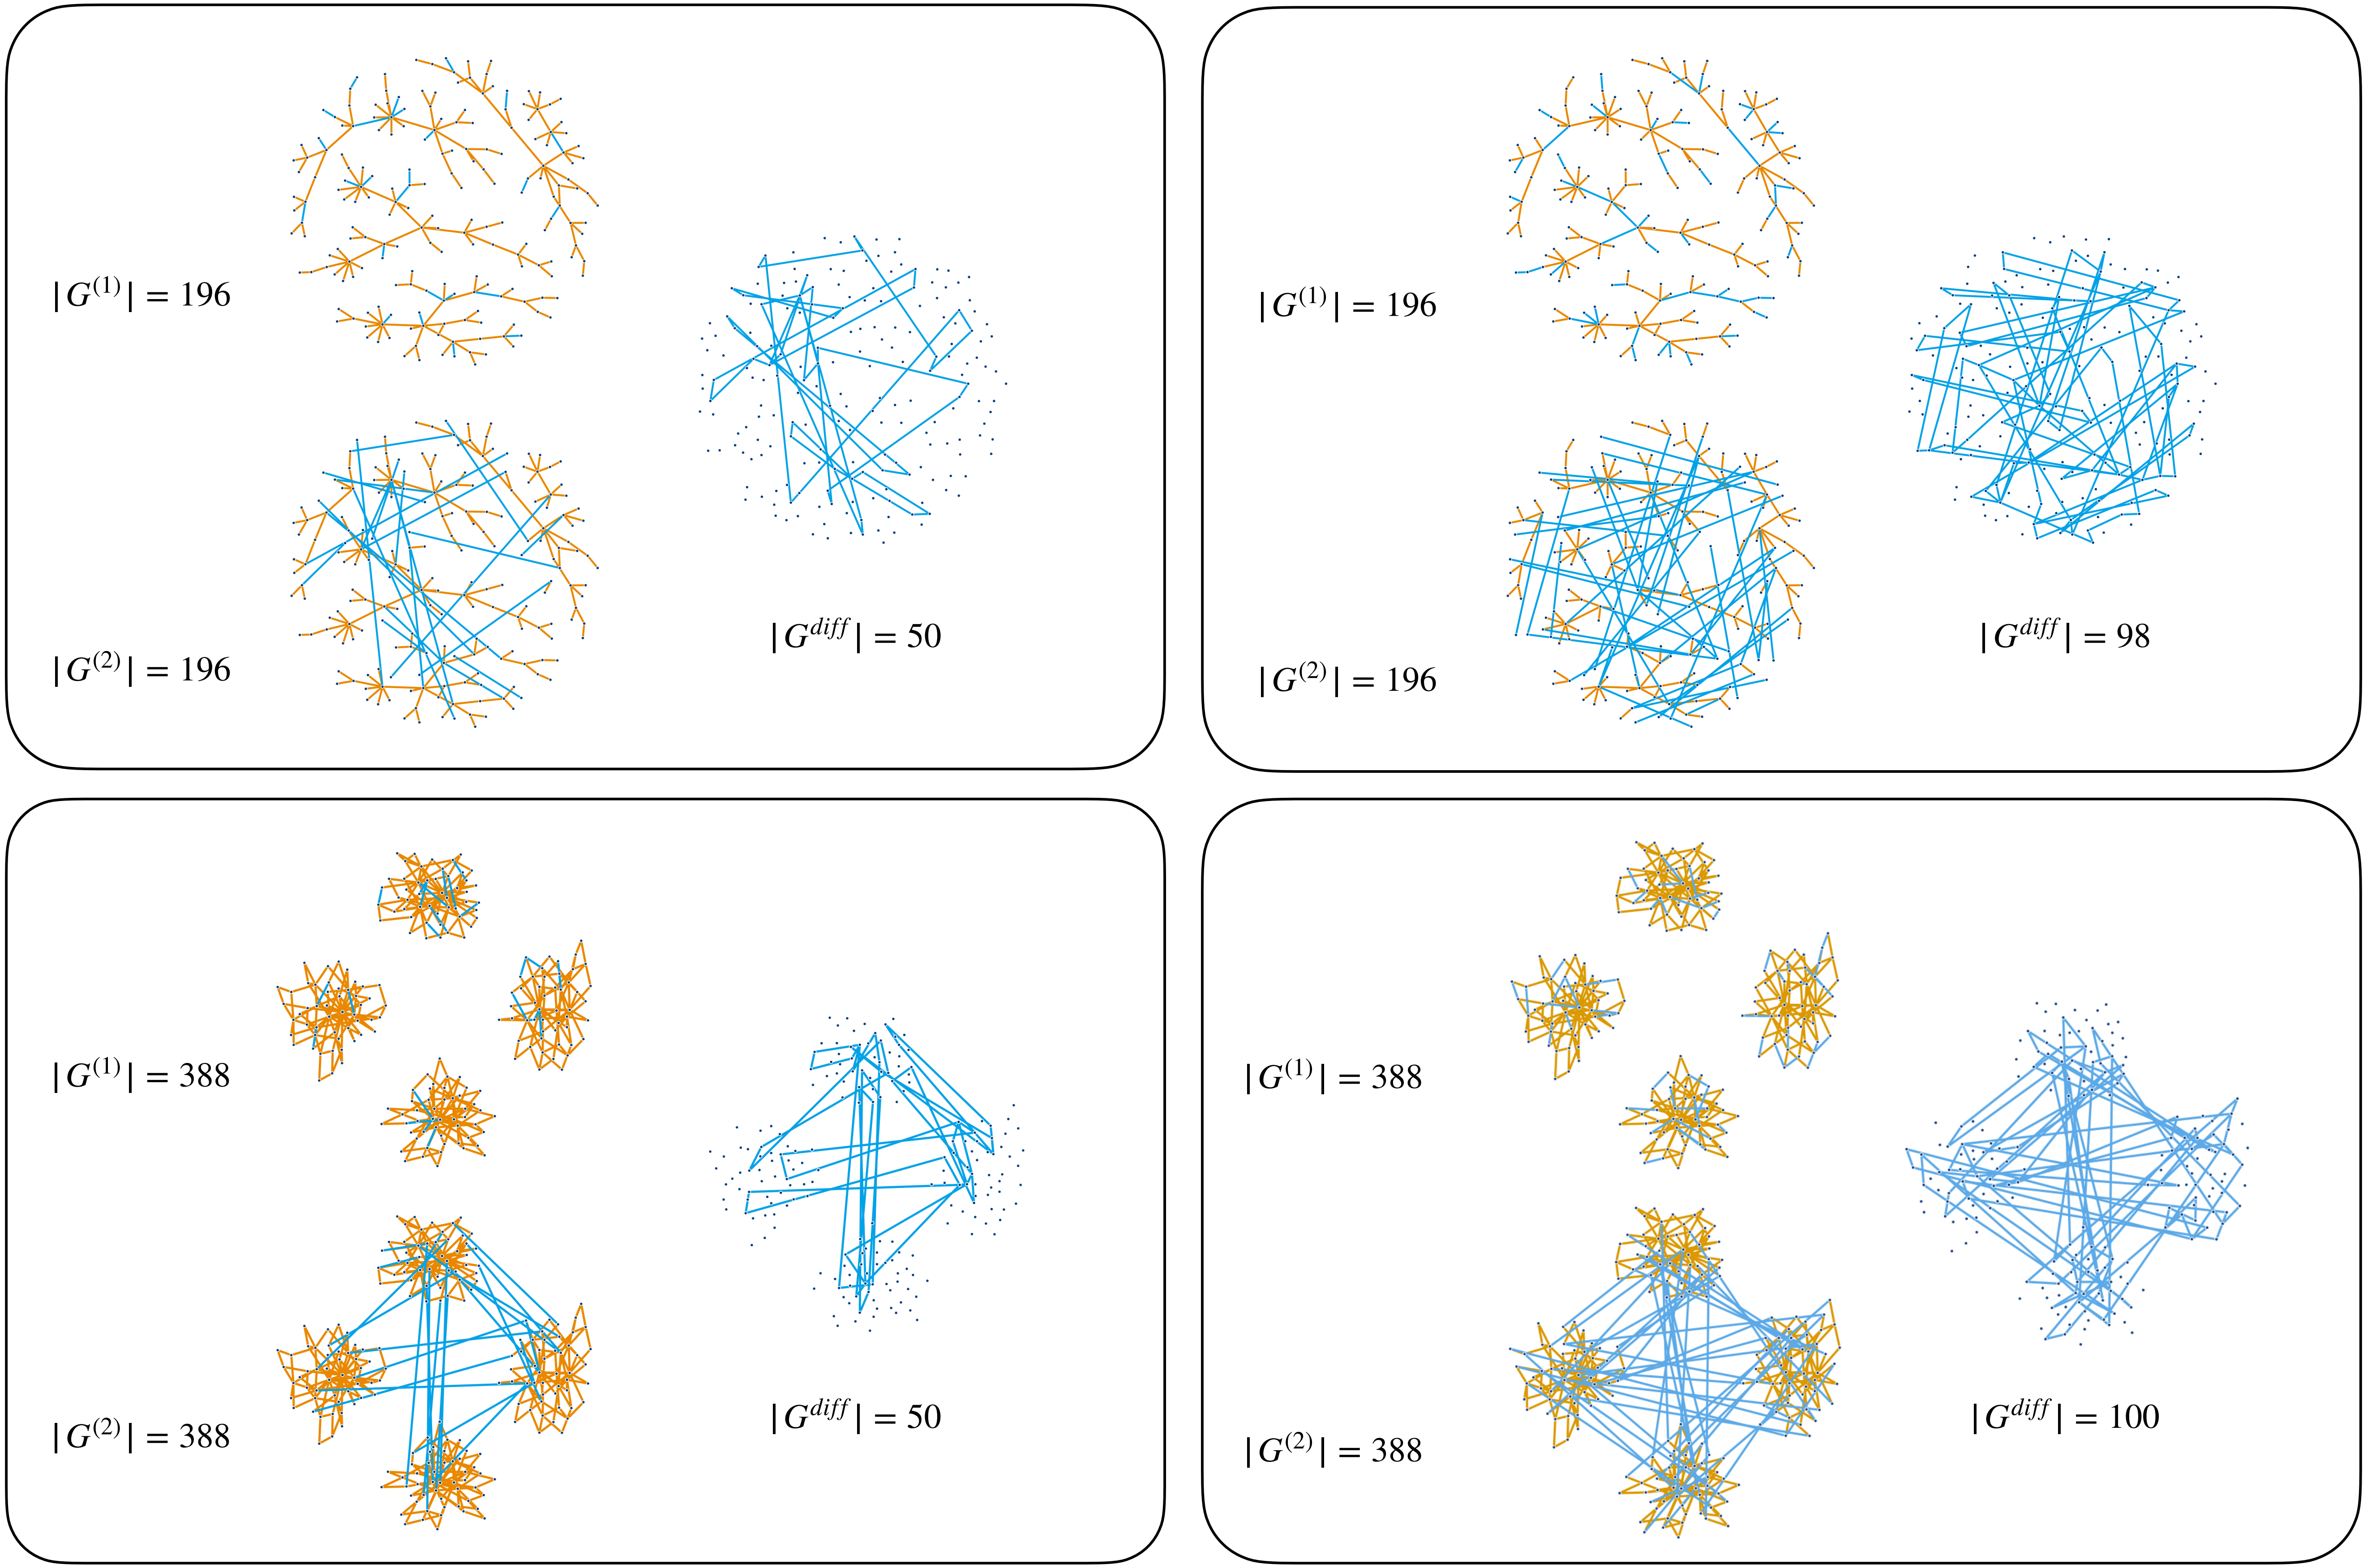

# Scale-free differential graph

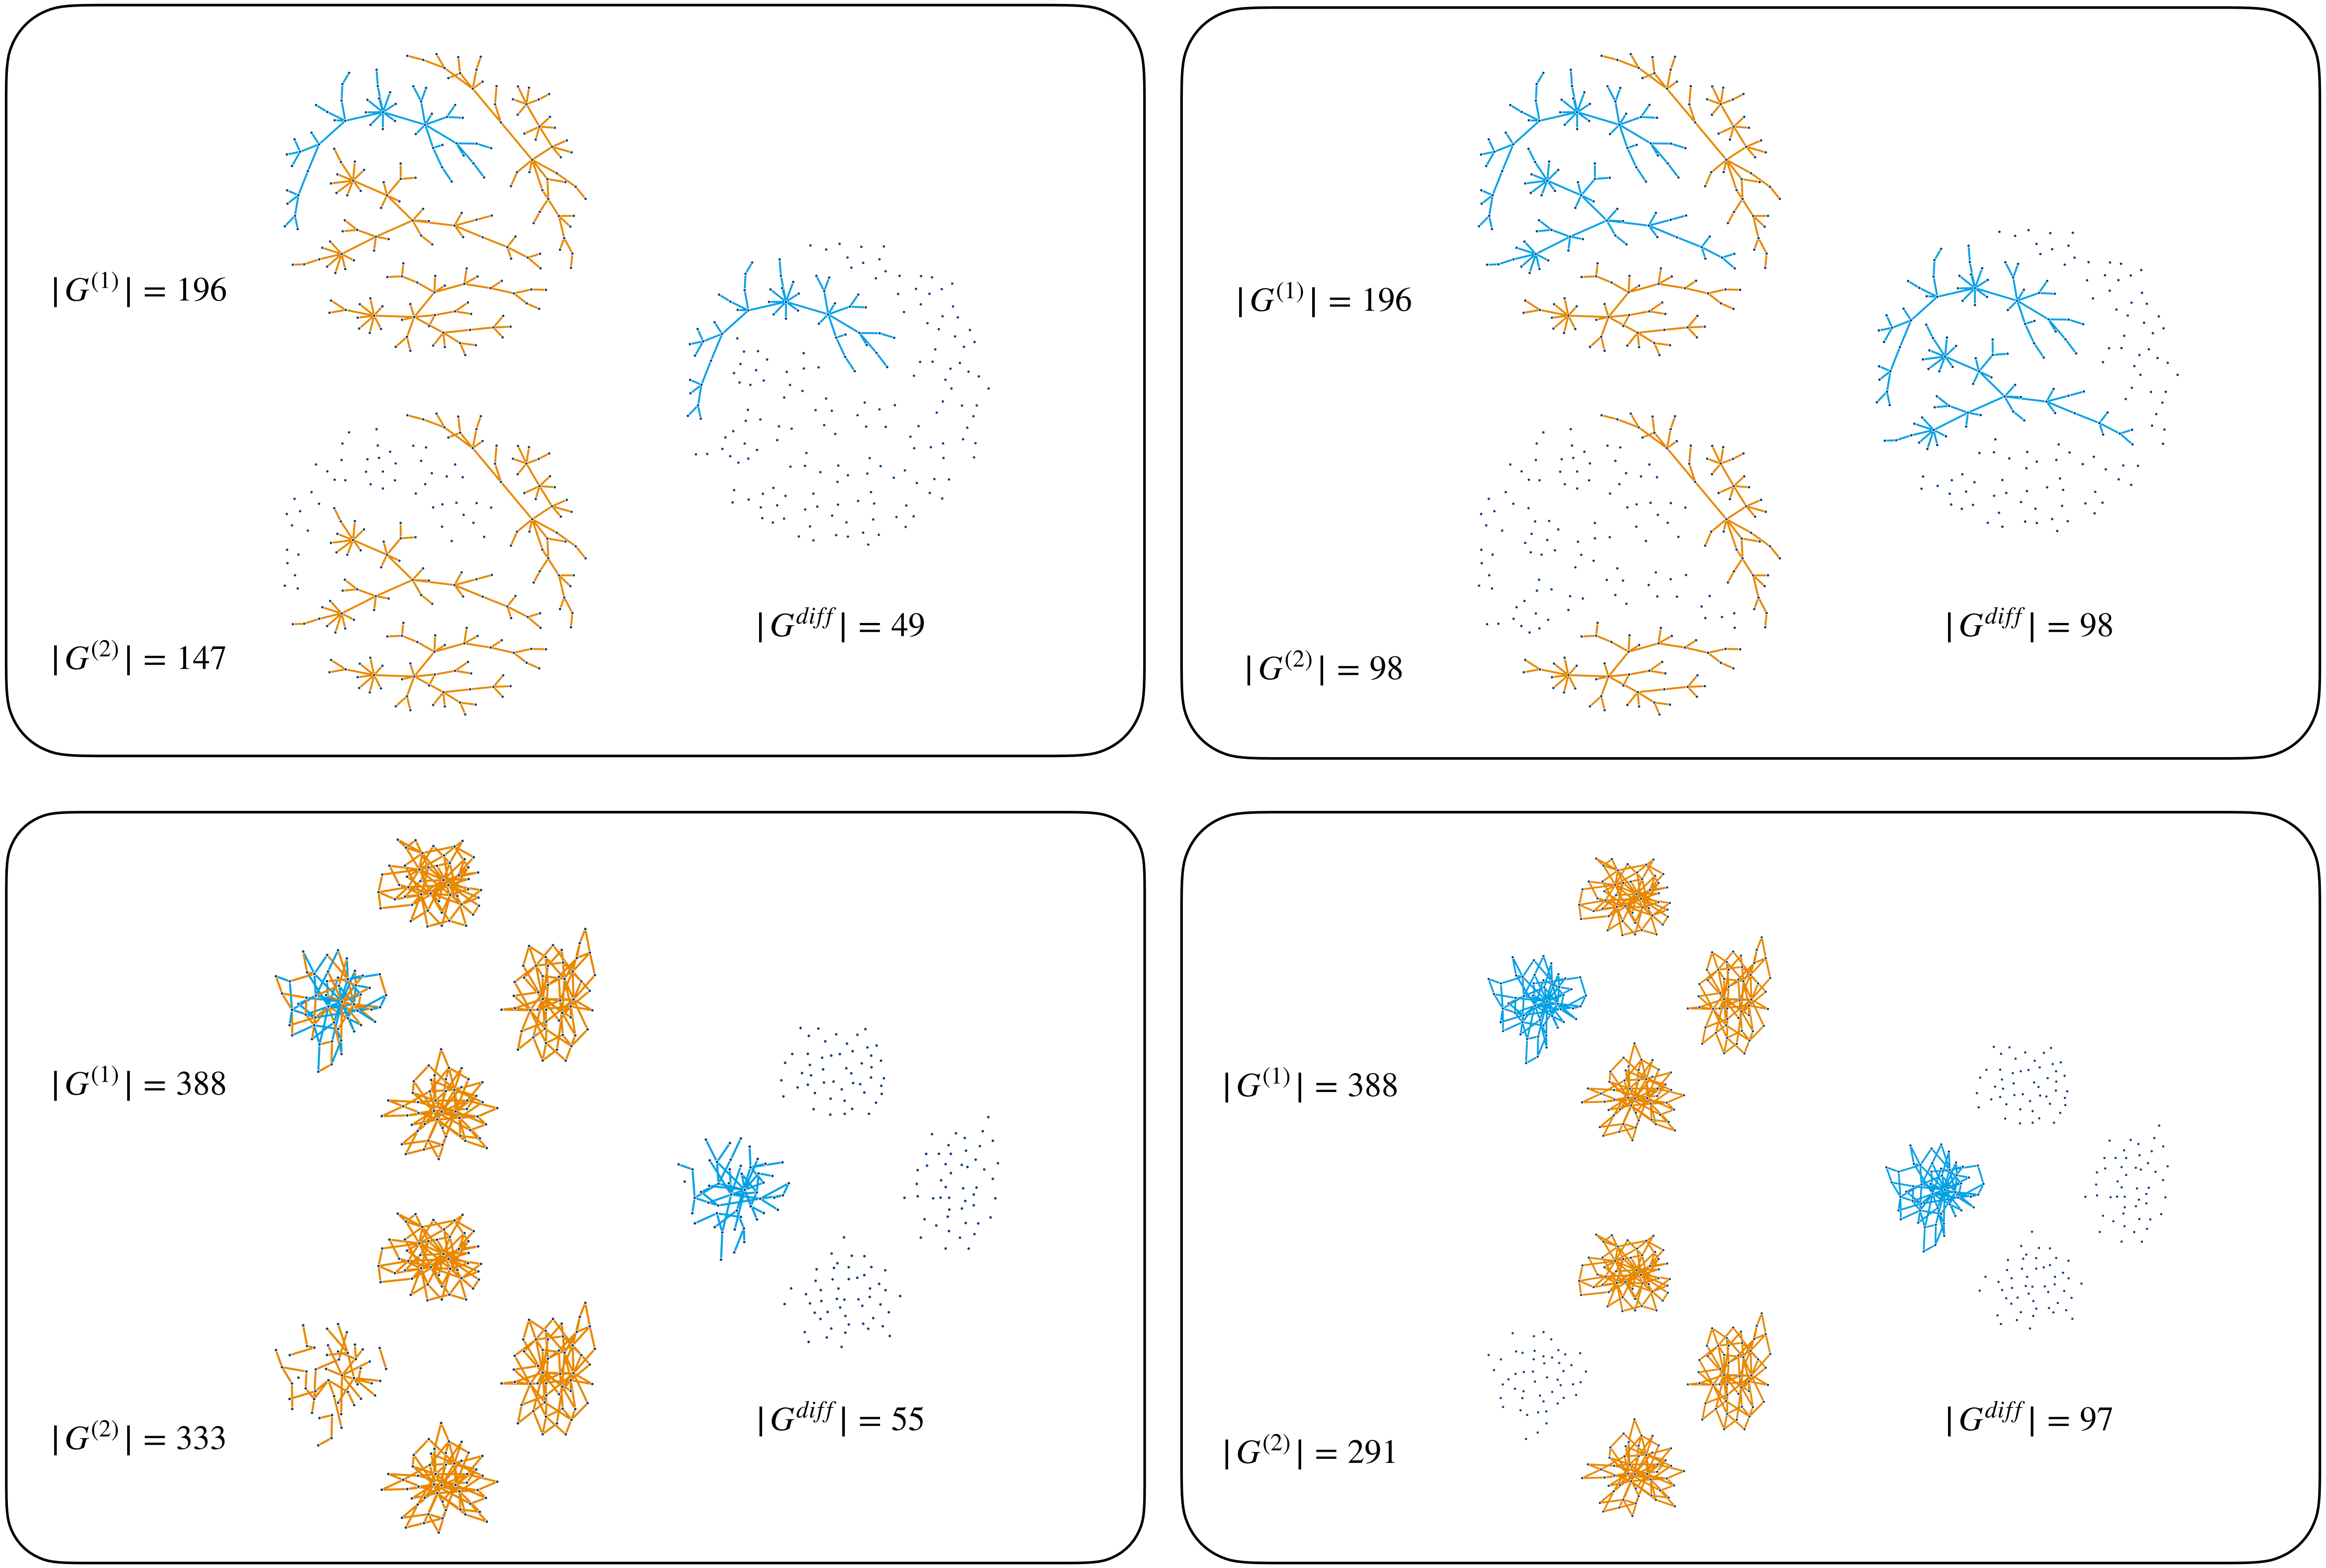

# Star differential graph

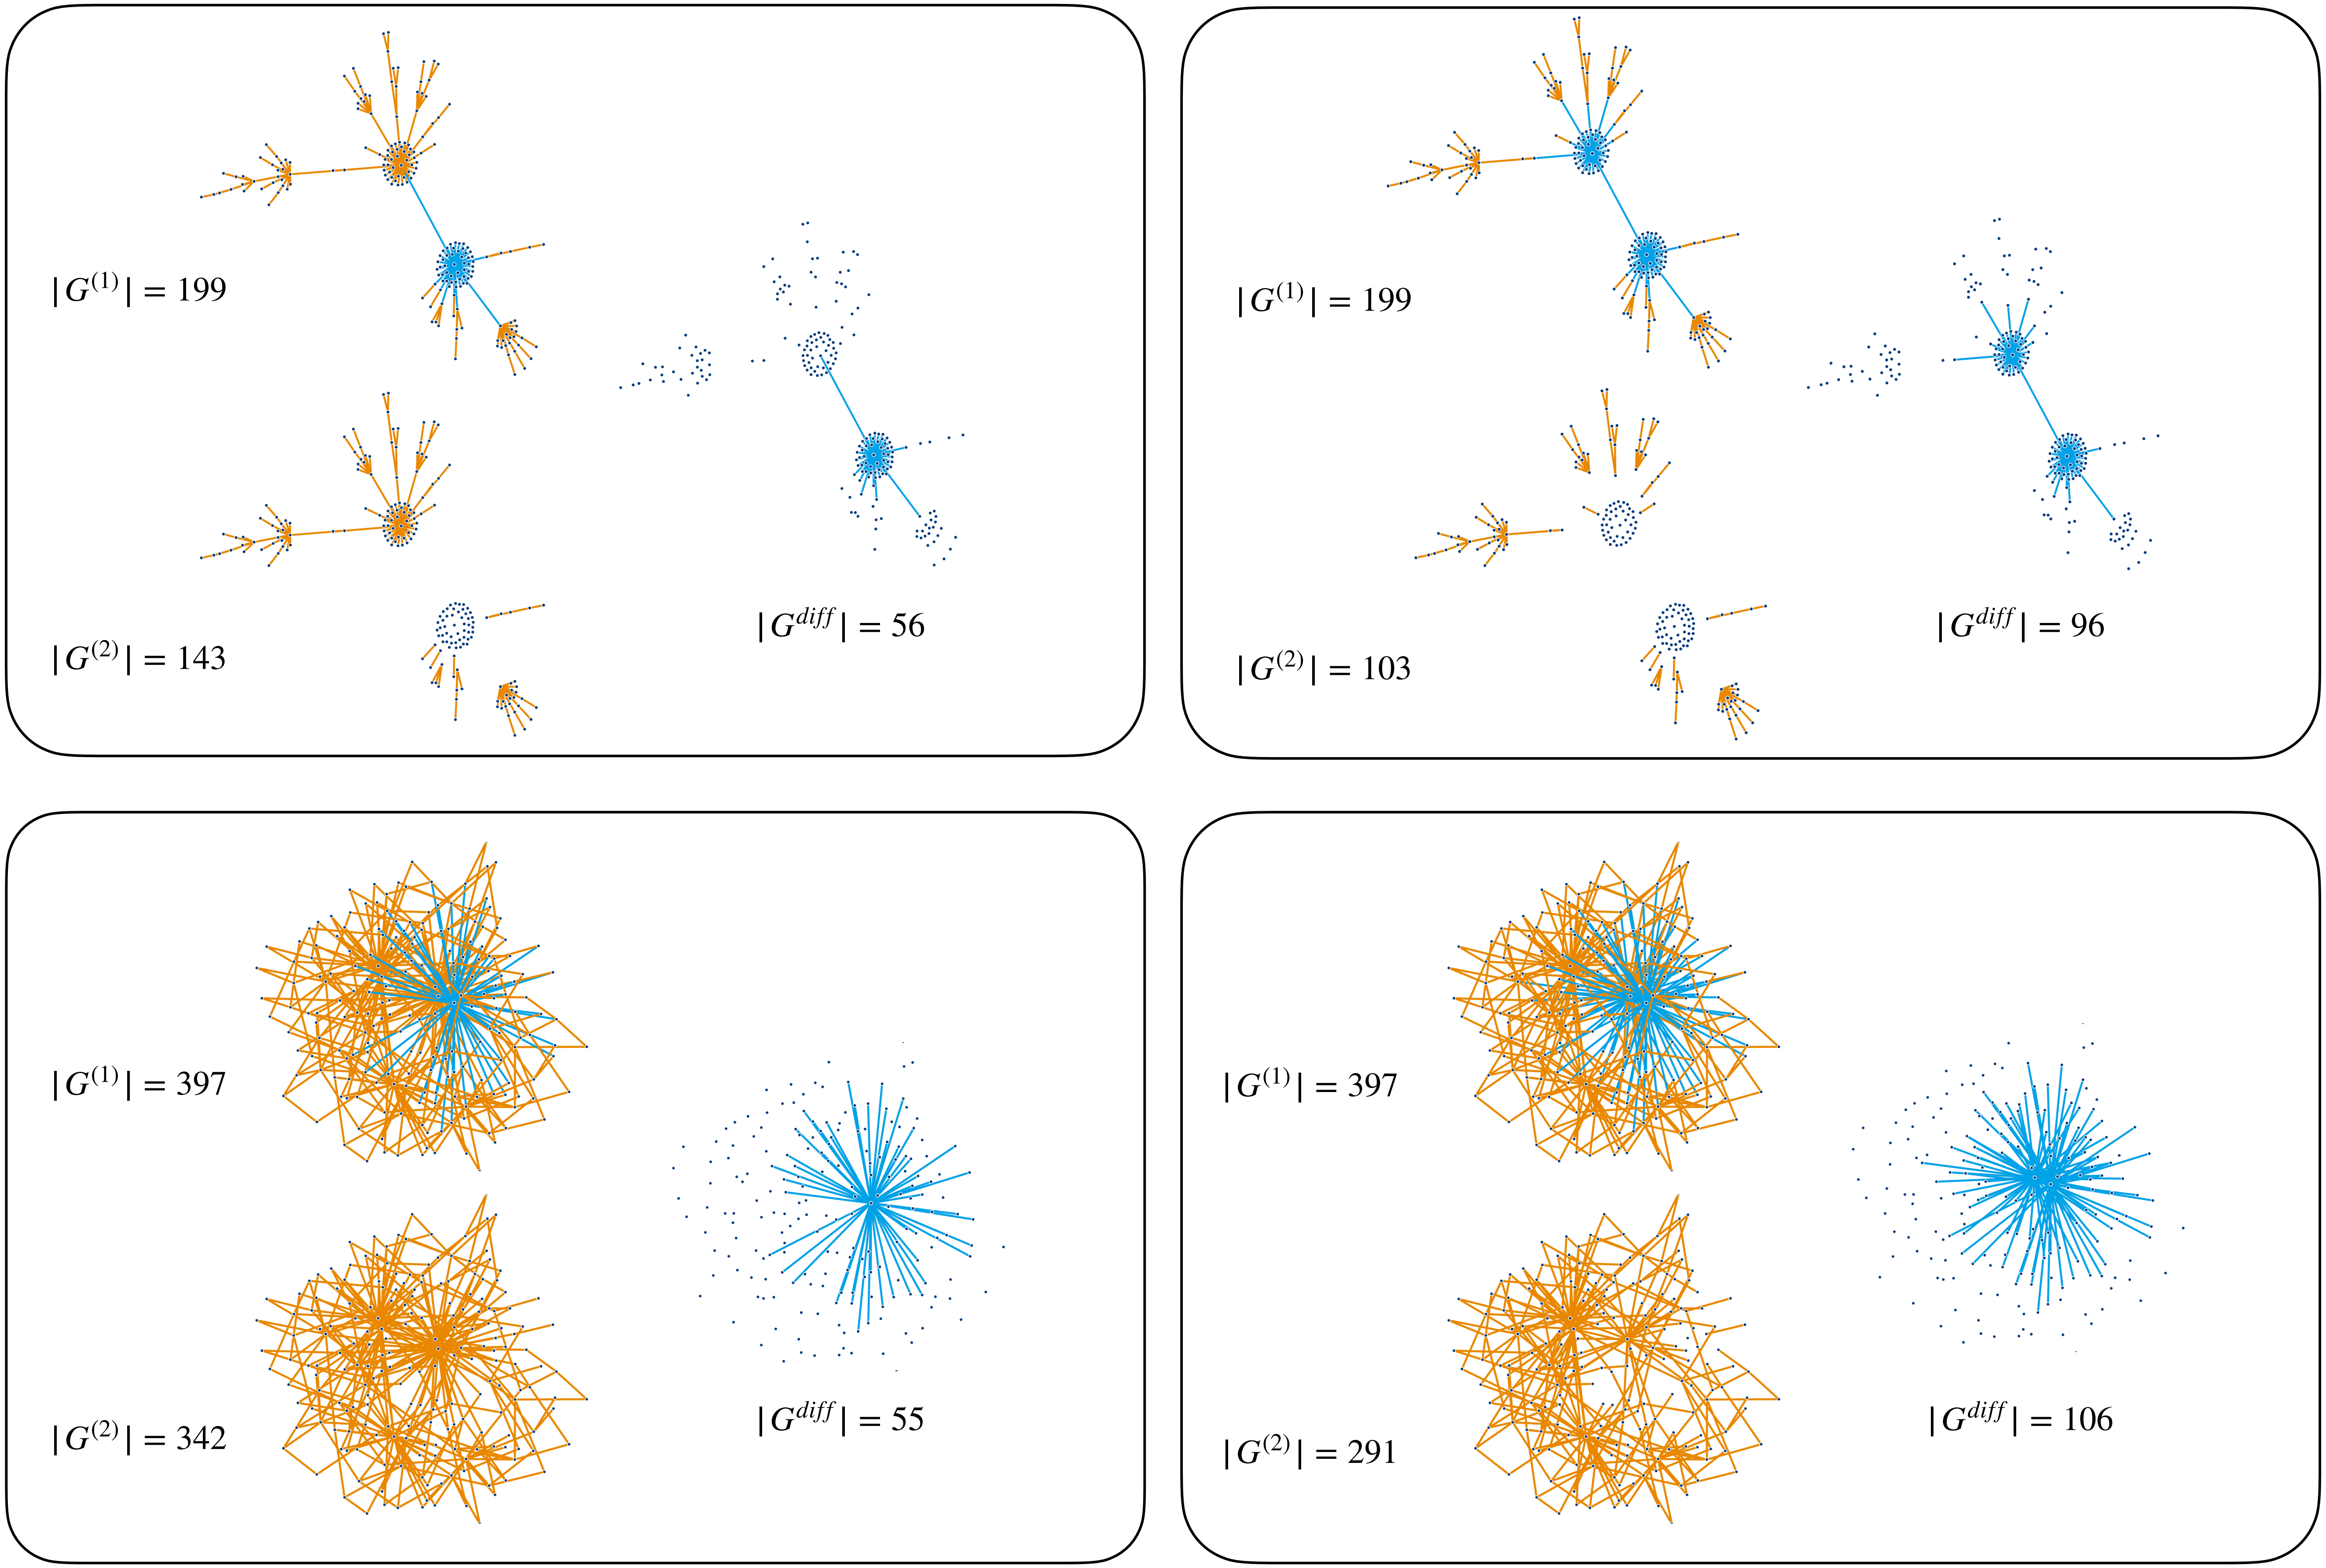

## Supplementary materials, Figure (b): $\alpha$ vs FDR

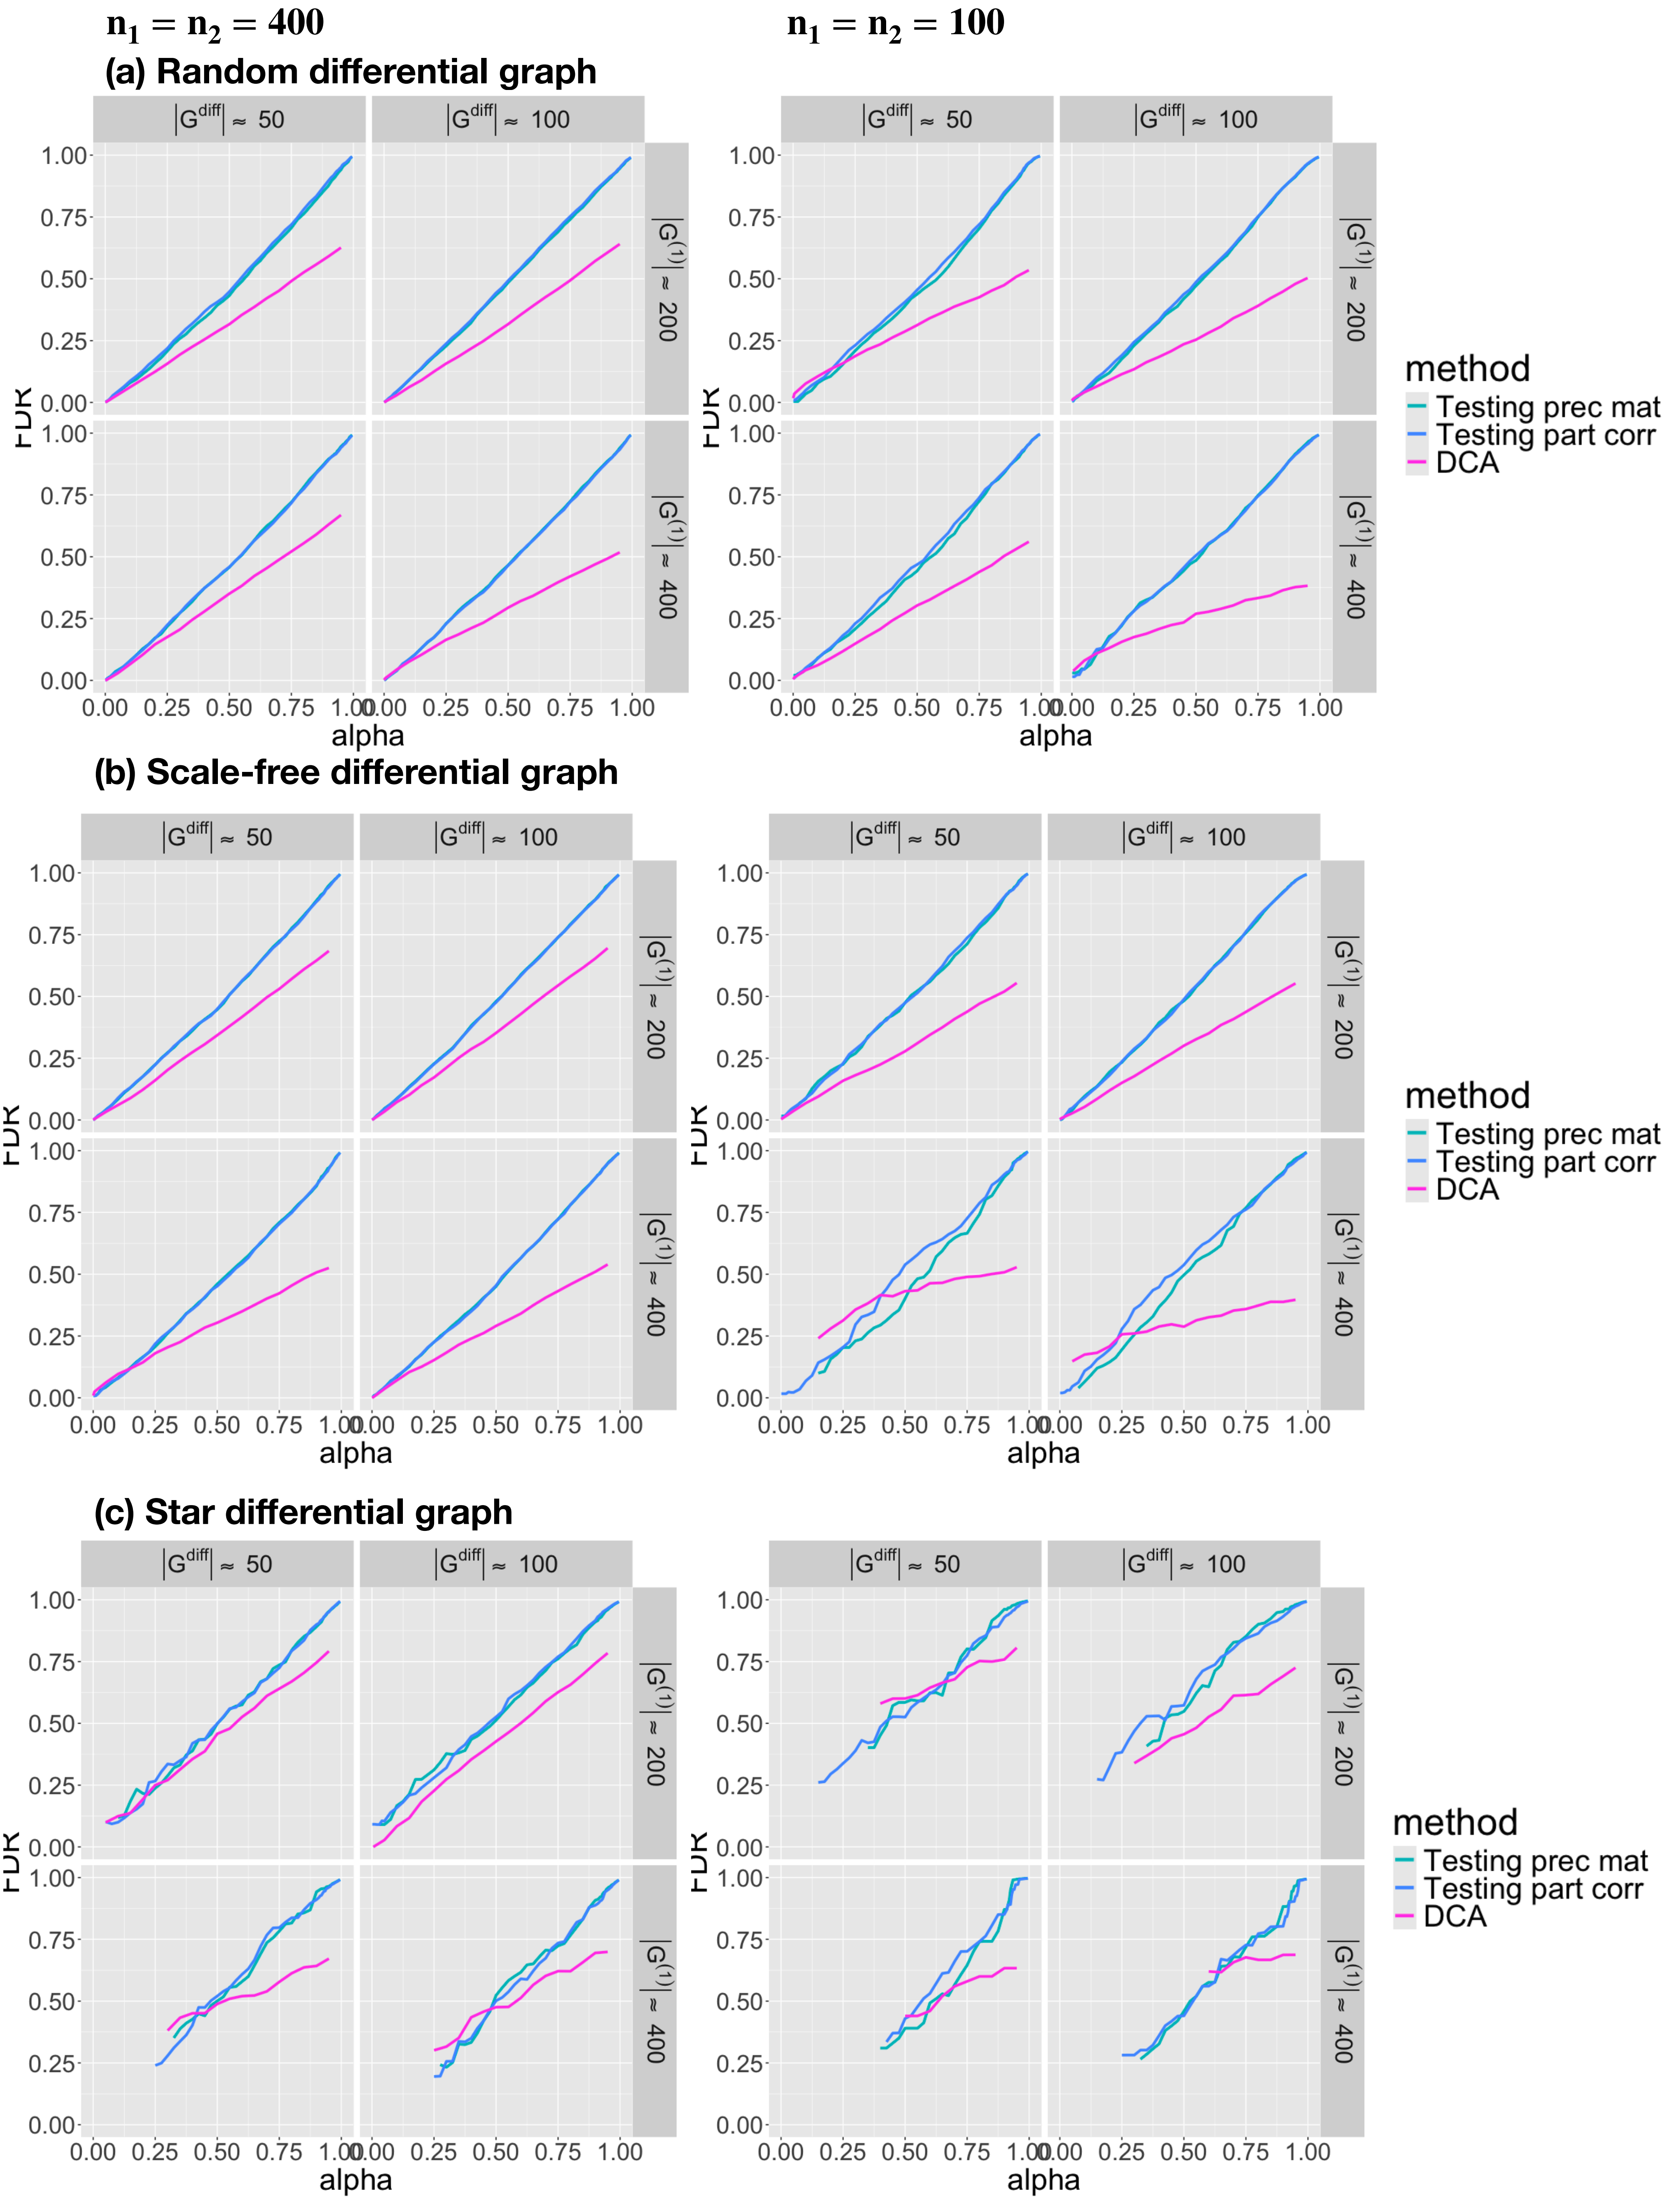

**Supplementary materials, Figure (c): sample size influence on performance**

We explored influence of large sample size on performance of a differential network estimation method based on **testing for equality of precision matrices entries**[1] (as it is quite fast compared to other methods in our simulation study). Results presented are for the star differential graph. Power vs FDR results are averaged over 50 realisations.

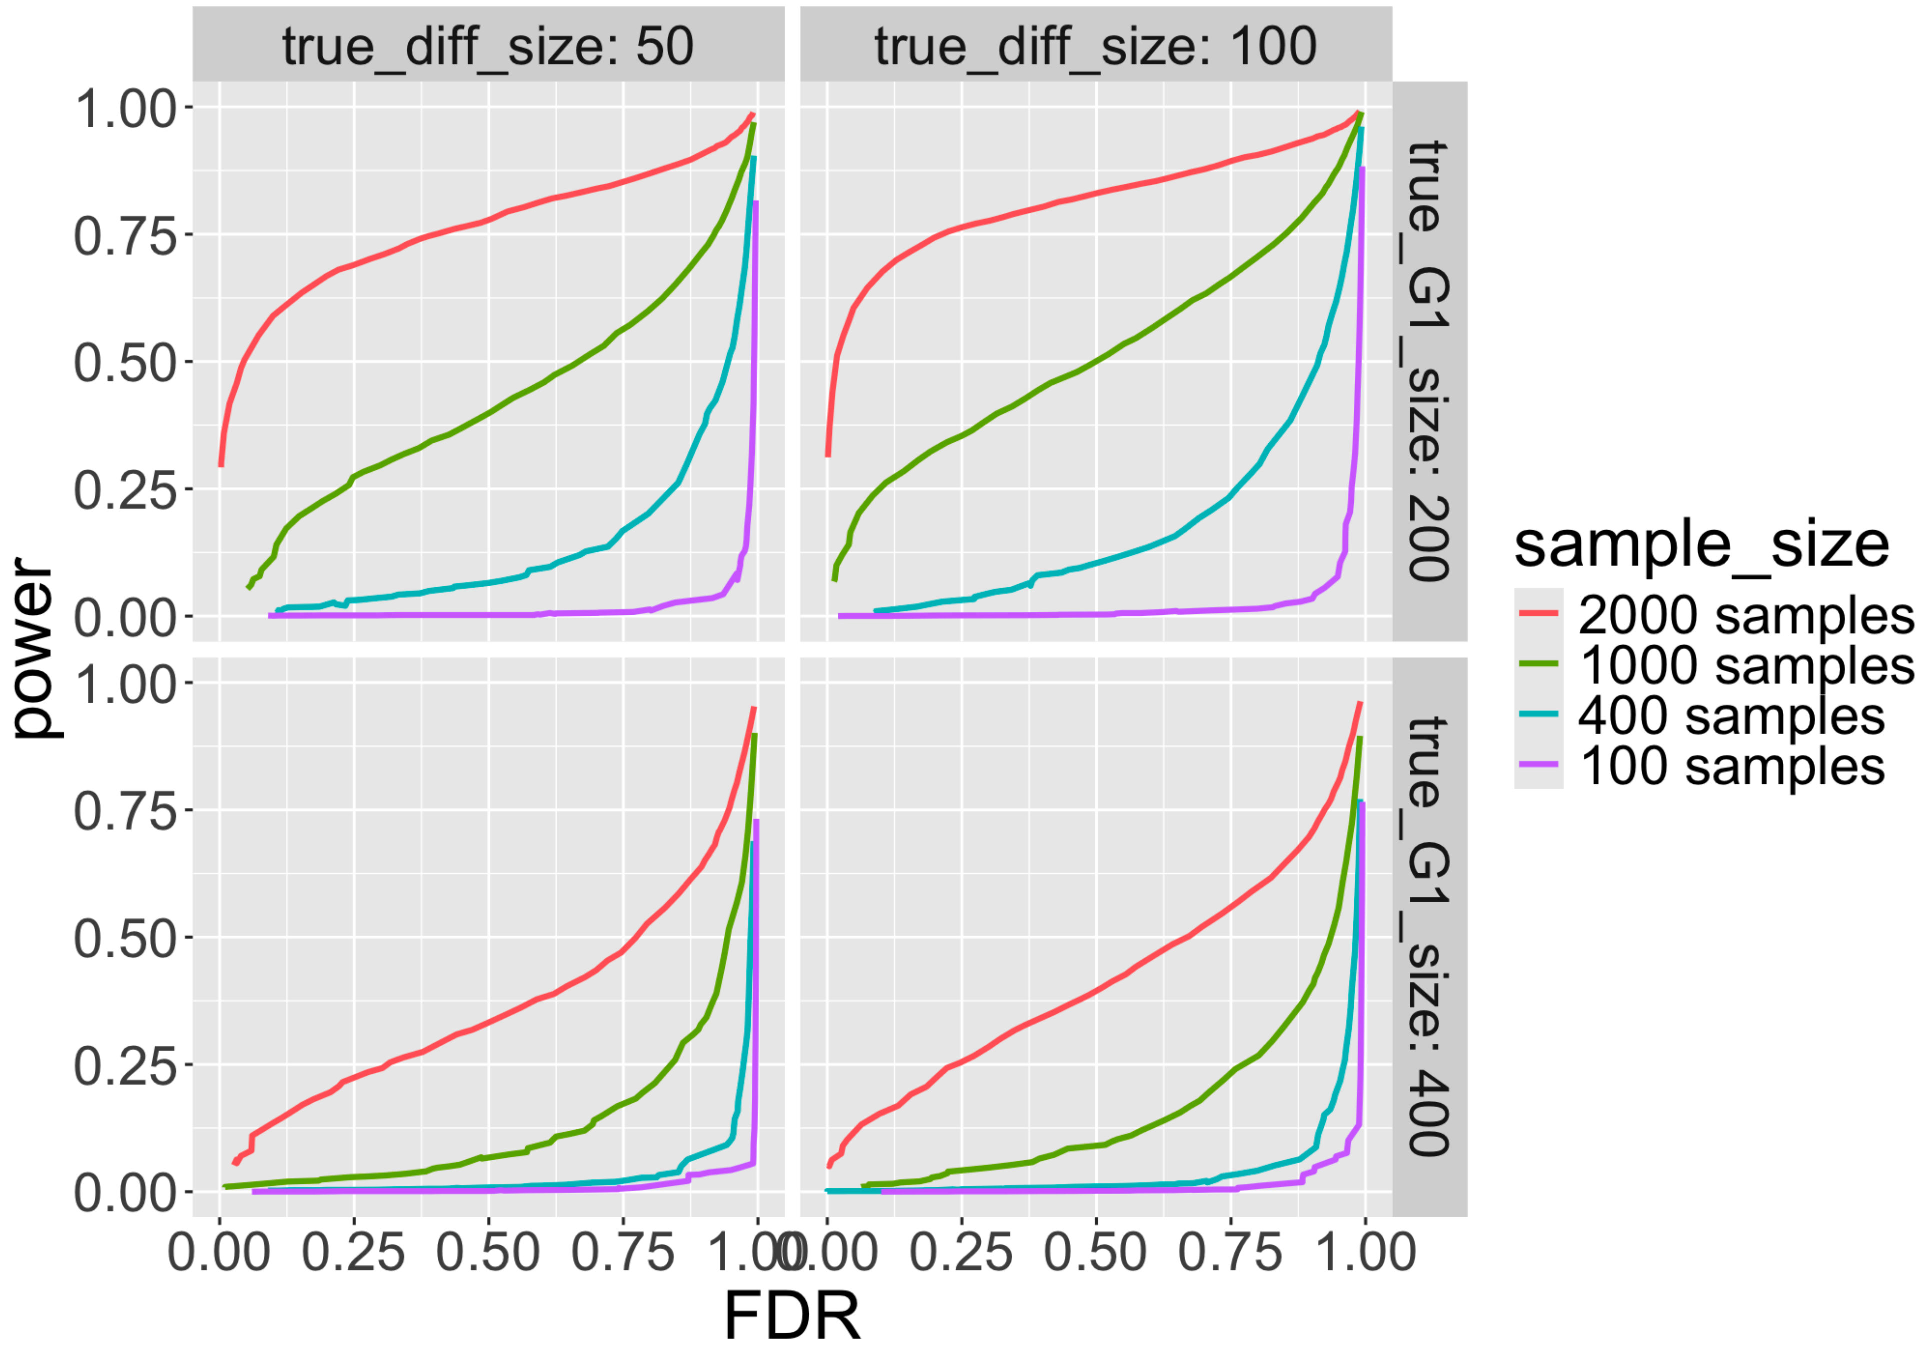


[1] Yin Xia, Tianxi Cai, and T. Tony Cai. Testing differential networks with applications to the detection of gene-gene interactions. Biometrika, 102(2):247–266, 6 2015
